# Supplementary material for: Out of equilibrium higher-order topological insulator: Floquet engineering and quench dynamics
Source: arXiv:1904.07247 source file (2020-01-01)
Supplement: Supplementary file 1 [file Supplementary_FlqHOTI_Reduced.pdf]

# Supplementary Material for "Out of equilibrium higher-order topological insulators: Floquet engineering and quench dynamics"

Tanay Nag,[1,2] Vladimir Juričić,[3] and Bitan Roy[2,4]

[1]SISSA, via Bonomea 265, 34136 Trieste, Italy

[2]Max-Planck-Institut für Physik komplexer Systeme, Nöthnitzer Str. 38, 01187 Dresden, Germany

[3]Nordita, KTH Royal Institute of Technology and Stockholm University, Roslagstullsbacken 23, 10691 Stockholm, Sweden

[4]Department of Physics, Lehigh University, Bethlehem, Pennsylvania, 18015, USA

(Dated: November 11, 2019)

In this Supplemental Material we show that the periodic appearances of the complete, partial and no revival in the survival probability of a topological corner mode of an initial (realized for $t < 0$) second order topological insulator at time $t > 0$, after a sudden quench at $t = 0$, such that the final state becomes a quantum spin Hall insulator, is insensitive to the group velocity in the system. Furthermore, we address (a) the survival probability and (b) the spectral density of the time evolved one-dimensional edge state for time $t > 0$, when an initial (realized for $t < 0$) quantum spin Hall insulator phase encounters a sudden quench at $t = 0$, such that for $t > 0$ the final system represents a higher order topological insulator, supporting only corner localized zero energy states.

In the main paper (MP), we discussed the quench dynamics of a two-dimensional HOT insulator. We showed the dynamics of the survival probability ($P_s$) and the spectral density of time evolved wavefunction at various instances for corner localized zero-energy modes at time $t > 0$, after a second order topological insulator encounters a sudden quench and at $t > 0$ the system describes a first order or quantum spin Hall insulator. We find that due to the presence of one-dimensional gapless helical modes in the final state, the corner mode dominantly propagates through the edges of the system, and the survival probability displays periodic appearances of complete, partial and no revival for long time after the quench (Fig. 4 of MP). Such repeating pattern of the survival probability is also anchored from the spectral density of the time evolved wavefunction (Fig. 5 of MP).

Two partial revivals take place at time $t = L/v_{\rm max}$ and $3L/v_{\rm max}$, no revival takes place $t = 2L/v_{\rm max}$, while a complete revival occurs $t = 4L/v_{\rm max}$. Later this pattern continues to appear periodically for a long time. Here,

$$v_{\rm max} = \frac{(1+m)t_0^2}{\sqrt{t_1^2 + (1+m)^2 t_0^2}} \tag{1}$$

is the maximum value of the group velocity and $L$ is the linear dimension of the system in $x$ and $y$ direction. The general expression for the group velocity along the $i$th direction, where $i = x, y$, is given by $v_i = \partial|E(\mathbf{k})|\partial k_i$, where $k_i$ is the $i$th component of the spatial momenta and $\pm E(\mathbf{k})$ are the energy spectra of the corresponding effective single-particle Hamiltonian, namely $H_{\rm SHI}$ [see Eq. (1) of MP]. As the $C_4$ symmetry is restored after the quench $v_x = v_y = v$ (say) for $t > 0$, and

$$E(\mathbf{k}) = \left[ t_1^2 \sum_{j=x,y} \sin^2 k_j + t_0^2 \left( m - \sum_{j=x,y} \cos k_j \right)^2 \right]^{1/2}. \tag{2}$$

The maximum value of the group velocity $v_{\rm max}$, is obtained for $\mathbf{k} = (1/2, 1)\pi$ or $\mathbf{k} = (1, 1/2)\pi$, see Eq. (1).

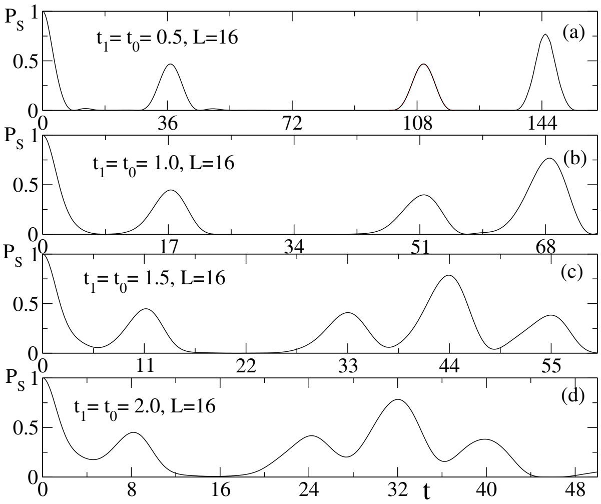


Figure 1: Dynamics of the survival probability ($P_s$) of a corner mode after a sudden quench at $t = 0$. The final state (at $t > 0$) is a quantum spin Hall insulator, supporting 1D counter propagating helical edge modes. Here, $L = 16$ is the linear dimension of the system in $x$ and $y$ directions. We tune the hopping parameters [namely, $t_1$ and $t_0$, keeping $m = 1$ throughout, see Eq. (1) of MP], yielding different values of $v_{\rm max}$, see Eq. (1). Irrespective of $v_{\rm max}$, two partial revivals ($P_s \approx 0.5$) occur at times $t = L/v_{\rm max}$ and $3L/v_{\rm max}$, no revival ($P_s \approx 0$) takes place at $t = 2L/v_{\rm max}$ and a complete revival ($P_s \approx 0.9$) at time $t = 4L/v_{\rm max}$, within one full cycle. At later time, this pattern continues to repeat itself. But, with increasing time the peak height of $P_s$ gradually decreases in each cycle. The pattern of the survival probability can be anchored from the spectral density of time evolved wavefucntion at various instances after the quench (see Fig. 5 of MP).

In Fig. 1 of the SM, we establish that the above mentioned pattern of the survival probability is insensitive to the precise value of $v_{\rm max}$. In particular, setting $m = 1$, we consider (a) $t_1 = t_0 = 0.5$, (b) $t_1 = t_0 = 1.0$, (c) $t_1 = t_0 = 1.5$ and (d) $t_1 = t_0 = 2.0$ in Fig. 1, which

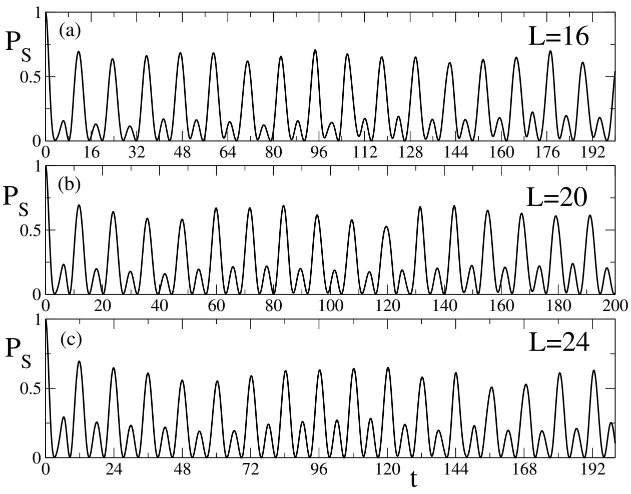


Figure 2: Dynamics of the survival probability ($P_s$) of one-dimensional helical edge mode at time $t > 0$, after a sudden quench at $t = 0$. For $t < 0$ ($t > 0$) the system describes a quantum spin Hall insulator (higher order topological insulator). Although the survival probability displays periodic appearances of complete, partial and no revival, their frequencies do not depend on the linear dimension of system in the $x$ and $y$ directions. We set $m = 1$ and $t_1 = t_0 = 1$. The corresponding spectral density of the time evolved wavefunction at various instances are shown in Fig. 3.

respectively yield (a) $v_{\max} \approx 0.45$, (b) $v_{\max} \approx 0.89$, (c) $v_{\max} \approx 1.34$ and (d) $v_{\max} \approx 1.79$, obtained from Eq. (1). We find that the complete, partial and no revival of the survival probability appears at the above mentioned times (almost) irrespective of $v_{\max}$.

In addition, we here discuss the similar effects after a quench at $t = 0$, such that for $t < 0$ the system describes a QSHI, while for $t > 0$ the final state represents a HOTI, supporting zero modes that are localized only at the corner (rest of the states at finite energies are localized in the bulk of the system). Such a quench dynamics can be addressed by choosing the following profile of the four-fold rotational ($C_4$) and time-reversal symmetry breaking perturbation [compare with Eq. (10) of MP]

$$V(t) = V_{12}\, \Gamma_4\, \Theta(t), \tag{3}$$

where $\Theta$ is the heaviside step function of its argument. Then the initial state describes a QSHI, supporting helical edge modes, while the final state describes a second order topological insulator. The dynamics of the survival probability of such an edge mode is shown in Fig. 2 and the corresponding spectral density of time evolved wavefunction at various instances is displayed in Fig. 3.

The survival probability in this situation also displays periodic appearances of the complete, partial and no revival. Since the final state supports localized zero-energy modes only at the corners (in contrast to the situation across the HOTI-QSHI quench, where the postquench phase supports gapless 1D edge modes), the propagation of an initial one-dimensional edge mode after the quench takes place through the entire system and it involves all (including bulk and corner) states. Also the gapless postquench corner states only occupy a tiny fraction of the entire system, thus only mildly affect the propagation of 1D edge states after the quench. Concomitantly, the spectral density of postquench the time evolved state considerably leaks into the bulk of the system, see Fig. 3, in contrast to the situation across the HOTI-QSHI quench where only a negligible a fraction of the spectral density diffuses into the interior of the system, see Fig. 5 of main text. These are possibly the reasons why the frequency of the complete, partial and no revival does not show any system size dependence, in contrast to the situation summarized in Fig. 1.

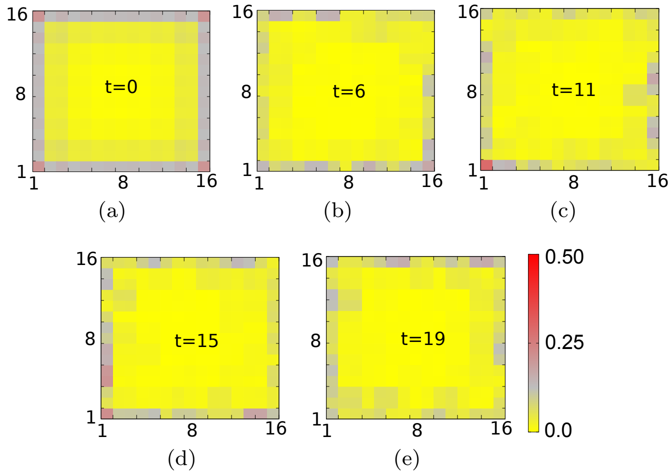


Figure 3: Spectral density of time evolved state $|\Psi(t)\rangle = \exp(-iH_{\rm Fin}t)|\Psi^{\rm initial}_{\rm edge}\rangle$ at time $t = 0$ and various instances after a sudden quench at $t = 0$ in a system with linear dimension $L = 16$ in both directions. Here, $|\Psi^{\rm initial}_{\rm edge}\rangle$ represents a one-dimensional edge mode, appearing in the spectra of the initial Hamiltonian $H_{\rm Ini} = H_{\rm SHI}$ [see panel (a)]. Since the final Hamiltonain $H_{\rm Fin} = H_{\rm SHI} + \Gamma_4 V_{12}$ accommodates zero-energy modes, localized only at the corners, propagation of the edge modes state at time $t > 0$ takes place through the entire system. This is possibly the reason why the frequency of complete, partial and no revival is insensitive to the system size, leading to the observed dynamics of the survival probability (see Fig. 2).
